# Supplementary material for: A Survey of Distributed Learning in Cloud, Mobile, and Edge Settings
Source: arXiv:2405.15079 source file (2024-05-23)
Supplement: Supplementary file 1 [file appendix.tex]

% Be sure to set \appendix or \appendices in structural/body.tex
% \chapter{Appendix Name}
% Text here.
% \section{Appendix section}
% Text here.
% \subsection{Appendix section}
% Text here.
% \subsubsection{Appendix section}
% Text here.
% \chapter{Another Appendix}
